# Supplementary material for: Probing the Melting of a Two-dimensional Quantum Wigner Crystal via its Screening Efficiency
Source: arXiv:1903.09949 ancillary file (2019-03-24)
Supplement: Supplementary file 1 [file WCC_SM_20190227.pdf]

# Supplemental Material to "Probing the Melting of a Two-dimensional Quantum Wigner Crystal via its Screening Efficiency"

H. Deng[1], L.N. Pfeiffer[1], K.W. West[1], K.W. Baldwin[1], L.W. Engel[2], and M. Shayegan[1]
[1]*Department of Electrical Engineering, Princeton University*
[2]*National High Magnetic Field Laboratory, Tallahassee, Florida*
(Dated: February 28, 2019)

In this Supplemental Material, we present additional details for our capacitance measurements of the screening efficiency of a two-dimensional electron system (2DES). We provide additional data for the 2DES at density $n = 4.2 \times 10^{10}$ cm$^{-2}$ (Section I), and also at $n = 6.0 \times 10^{10}$ cm$^{-2}$ (Section II). In Section III we discuss a circuit model for our capacitance measurements.

## I. ADDITIONAL DATA FOR $N = 4.2 \times 10^{10}$ CM$^{-2}$

In Fig. S1, we present the experimental data for the magnetic field ($B$) dependence of the penetration current ($I_P$) at different temperatures ($T$). For clarity, we show only selected traces at representative $T$ in Fig. S1. The complete set of experimental data, with smaller steps in $T$, is used to construct the color-density map of Fig. 2(a). As described in the manuscript, the fractional quantum Hall states (FQHSs), e.g., at filling factors $\nu = 2/9$ or 1/5, show maxima in $I_P$, originating from the incompressibility of the FQHS. Because the $\nu = 2/9$ FQHS is weak in our sample, $I_P$ at $\nu = 2/9$ shows only a small bump rather than a well-developed peak. At low $T$, the Wigner crystal (WC) at $\nu < 1/5$ and the reentrant Wigner crystal (RWC) at $\nu = 0.21$ (green triangle in Fig. 1 and Fig. S1) also show high values of $I_P$, because the pinned electron crystal has an insulating behavior and therefore low screening efficiency. Between the WC/RWC and nearby FQHSs, there are three $I_P$ minima (red triangles in Fig. 1), which are the key observations of our work.

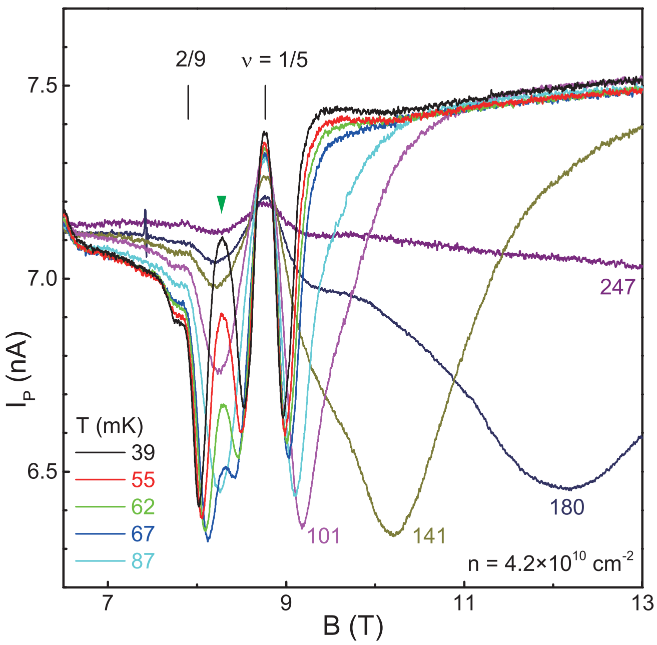


FIG. S1. Magnetic field dependence of $I_P$ at different temperatures for $n = 4.2 \times 10^{10}$ cm$^{-2}$. The values of temperature are noted on the lower-left table or near the traces with corresponding colors. The green triangle indicates the position of the reentrant Wigner crystal.

Regarding the RWC, with increasing $T$, the $I_P$ peak of the RWC decreases, and the two $I_P$ minima flanking the RWC approach each other, until the $I_P$ peak completely disappears at $T \simeq 77$ mK (Fig. S1). At higher temperatures, $I_P$ at $\nu = 0.21$ increases monotonically with $T$. This evolution leads to the "dome" structure of the

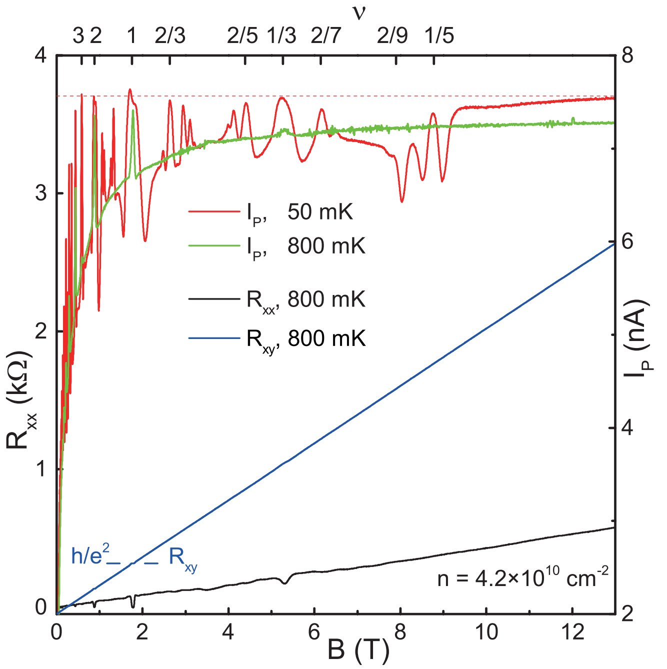


FIG. S2. Results of transport and penetration current measurements at high $T$. The black trace is the longitudinal magnetoresistance ($R_{xx}$) and the blue trace is the Hall resistance ($R_{xy}$). The value of $h/e^2$ is indicated by the blue horizontal lines around the very narrow $R_{xy}$ plateau at $\nu = 1$. The red and green traces are the penetration current ($I_P$) measured at low and high $T$. The red, dashed horizontal line indicates the maximum value of $I_P$ at low $T$.

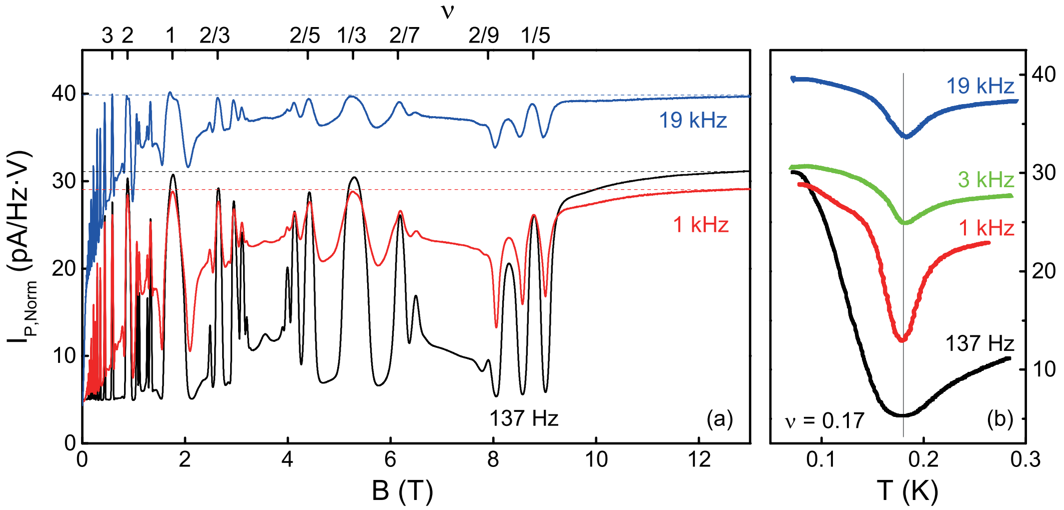


FIG. S3. (a) Magnetic field dependence of $I_P$ measured at different frequencies of $V_{AC}$ for the 2DES at $n = 4.2 \times 10^{10}$ cm$^{-2}$. $I_P$ is normalized by the frequency and the amplitude of $V_{AC}$. The dashed horizontal lines indicate the maximum values of $I_P$ at different frequencies. (b) Temperature dependence of $I_P$ measured with different $V_{AC}$ frequency at $\nu = 0.17$.

$I_P$ minima which encloses the RWC regime in Fig. 2(a). At the same time, the $I_P$ minimum between the $\nu = 1/5$ FQHS and the WC at lower-$\nu$ side moves to higher $B$ positions with increasing $T$, resulting in the "valley" of $I_P$ minima between the WC and liquid phase of the 2DES for $\nu < 1/5$ in Fig. 2(a).

In Fig. S2, we present both transport and $I_P$ measurement results at high $T$ ($\simeq 800$ mK); for comparison, we also show the $I_P$ trace at $T = 50$ mK. The longitudinal magnetoresistance ($R_{xx}$) shows a gradual increase with $B$. Only the strongest quantum Hall states (QHSs) at $\nu = 2, 1$ and $1/3$ survive as shallow $R_{xx}$ minima. Correspondingly, the Hall resistance ($R_{xy}$) exhibits essentially a classical (linear) Hall effect, with very weak and narrow plateaus at $\nu$ of the strong QHSs. Also, $I_P$ at such high $T$ shows fewer features compared to its low-$T$ counterpart. $I_P$ peaks of the weak QHSs disappear, and those for the strong QHSs ($\nu = 2, 1, 1/3$, etc.) become narrower and lower. Note that, in a large high-$B$ range ($> 7$ T), $I_P$ attains an almost constant value which is lower than $I_P$ of the strong FQHSs and WC at low $T$. This value is essentially the saturated $I_P$ value at high $T$ observed in the $T$-dependence measurements described in the manuscript [Figs. 2(d) and 2(e)]. We suspect that, the 2DES is highly excited above its the ground states (i.e., FQHSs and WC) at such high $T$, becoming a highly correlated liquid phase which has a nearly constant screening efficiency in a large range of $B$.

In Fig. S3, we present the measured $I_P$ vs $B$ and $T$ traces at multiple $V_{AC}$ frequencies. We used frequencies from 137 Hz to 19 kHz, covering $\sim 2$ orders of magnitude. For convenience, $I_P$ is normalized by the frequency and amplitude of $V_{AC}$. As Fig. S3(a) shows, although the $B$ dependence of $I_P$ measured at different frequencies has a different magnitude, all the traces of $I_P$ are qualitatively similar: the QHSs result in $I_P$ peaks, the compressible Fermi liquid phases have lower $I_P$, and the WC/RWC show larger $I_P$. Also, for each frequency, the strong QHSs and WC states have almost the same maximum value of $I_P$ [dashed line for each trace in Fig. S3(a)]. As we discussed in the manuscript, for any state of the 2DES with minimal screening efficiency, $I_P$ shows a maximum value corresponding to the geometric capacitance between the top and bottom gates.

Ideally, after the normalization by the frequency and amplitude of $V_{AC}$, all the $I_{P,Norm}$ traces in Fig. S3(a) are expected to have the same maximum value for the strong QHSs and WC states. However, in our experiments, because of the frequency response of our measurement circuit, the signal gain varies depending on frequency, leading to different $I_P$ maximum values after normalization for different frequencies. Also, Fig. S3(a) traces show an offset at zero magnetic field. Such an offset is not expected in an ideal setup because the 2DES at zero field is highly compressible and should fully screen the electric field leading to $I_P \simeq 0$. We suspect that the non-ideal, parasitic capacitances, e.g., the stray capacitance at the sample's edges or the capacitance between wires, cause this offset. We emphasize that Fig. S3(a) $I_P$ vs $B$ traces taken at different frequencies all show qualitatively a similar behavior, namely maxima and minima at the same fillings. In particular, $I_P$ minima separating the $\nu = 2/9$ and $1/5$ FQHSs, and the RWC and WC, are observed in all the traces.

It is important to note that the non-monotonic behavior of $I_P$ in the $T$-dependence measurements is also seen for all the frequencies. In Fig. S3(b), we present $I_P$ vs $T$ traces at $\nu = 0.17$ measured at different $V_{AC}$ frequencies. All the traces show that $I_P$ decreases with increasing $T$, reaches its minimum at a critical temperature ($T_C$), then increases at higher $T$. Moreover, all the traces show essentially the same $T_C$ for the $I_P$ minimum.

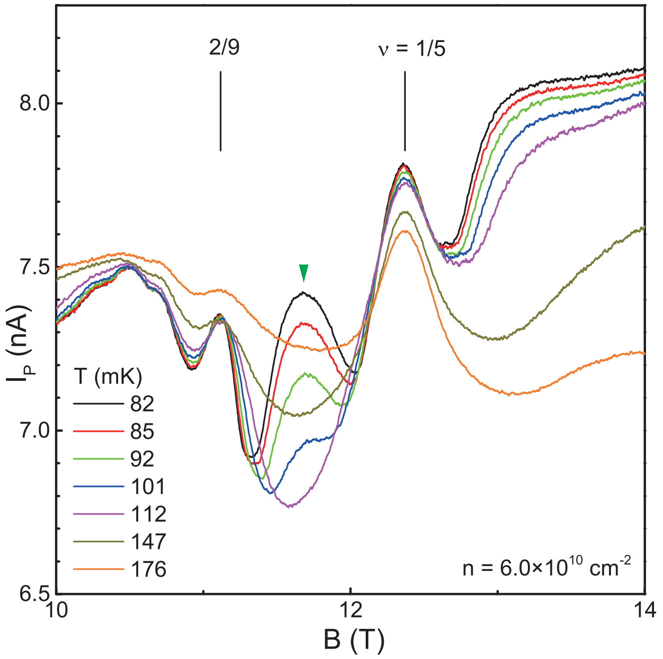


FIG. S4. Magnetic field dependence of $I_P$ at different temperatures for $n = 6.0 \times 10^{10}$ cm$^{-2}$. The values of temperature are noted on the lower-left table. The green triangle indicates the position of the reentrant Wigner crystal.

In both sets of independent measurements [Figs. S3(a) and S3(b)], the data taken at multiple $V_{AC}$ frequencies indicate that the $I_P$ minima seen between the FQHSs and WC/RWC in $B$-dependence measurements, and the minima at $T_C$ in $T$-dependence measurements, are unlikely to be artifacts of our experimental set-up or the measurement circuit. Rather, these $I_P$ minima are intrinsic properties of the 2DES.

## II. DATA FOR $N = 6.0 \times 10^{10}$ CM$^{-2}$

In Fig. S4, we present data for the $B$ dependence of $I_P$ at different $T$ for the 2DES at $n = 6.0 \times 10^{10}$ cm$^{-2}$. As described in the manuscript, we applied the same analysis to this batch of data and extracted $T_C$ plotted as blue circles in Fig. 3.

## III. CIRCUIT MODEL FOR CAPACITANCE MEASUREMENTS

In this Section, we present a circuit model for our capacitance measurements. As Fig. S5 shows, our measurement setup has a 3-terminal configuration. The AC signal source, i.e., $V_{AC}$, is coupled to the circuit through the geometrical capacitor between the bottom gate and the 2DES ($C_B$). After crossing $C_B$, the current is distributed into two branches. In one branch (the 2DES branch), the current is conducted through the 2DES to the ground, corresponding to the electric field screened by the 2DES. In the other branch (the $C_T$ branch), the current goes to the ground through the top-gate capacitor $C_T$; this corresponds to the penetration electrical field ($E_P$) reaching the top gate. Because the AC impedance of $C_B$ is significantly larger than the $C_T$ impedance, $V_{AC}$ and $C_B$ together could be treated as a near-constant current source. The distribution of the current after $C_B$ depends on the impedances of the 2DES and $C_T$ branches. It is intuitive that, when the impedance of 2DES branch is larger than the one of $C_T$ branch, $I_P$ would be high, and vice versa. Moreover, because $C_B$ and $C_T$ are fixed by the sample geometry, any change of $I_P$ reflects the change of the impedance of 2DES branch.

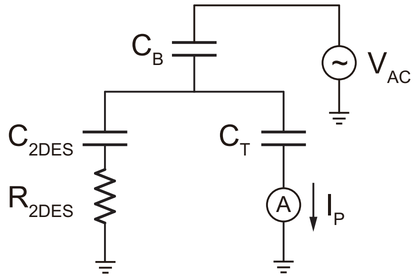


FIG. S5. The diagram of the circuit model for the capacitance measurements. $C_B$ ($C_T$) is the geometrical, parallel plate capacitor between the bottom (top) gate and the 2DES. $R_{2DES}$ and $C_{2DES}$ are the resistance and (quantum) capacitor of the 2DES respectively. $V_{AC}$ is the AC voltage applied on the bottom gate. $A$ is the lock-in amplifier in ammeter mode, which measures the penetration current $I_P$ crossing $C_T$

There are several possible components of the impedance in the 2DES branch. An obvious component is the 2DES resistance, which is represented as $R_{2DES}$ in Fig. S5. When the 2DES is in either strong QHSs or WC states, the bulk of 2DES is nearly insulating and therefore shows very high resistance. The screening efficiency of 2DES is essentially zero and almost all the current goes through the $C_T$ branch, leading to a high $I_P$. When the 2DES is in a highly conductive state, i.e., compressible states between the QHSs or the liquid state at low fillings after WC melts at high $T$, the screening efficiency is high, and therefore a low $I_P$ would be measured in $C_T$ branch. However, as discussed in the manuscript, the variation of $R_{2DES}$ alone is not enough to explain the experimental data: $R_{2DES}$ decreases monotonically during the melting of the WC when $T$ increases, resulting in only a monotonic increase of $I_P$. But the experimental data show that $I_P$ has a clearly non-monotonic behavior [Figs. 2(d) and (e)].

Therefore, we consider that the (quantum) capacitance of 2DES is another important component of the impedance in the 2DES branch ($C_{2DES}$ in Fig. S5). In order to lead to the non-monotonic behavior of $I_P$ with increasing $T$, the $T$ dependence of $C_{2DES}$ in the WC regime should be non-monotonic. As discussed in the manuscript, Ref. [26] provides a possible theoretical

explanation for the non-monotonic behavior of $C_{2DES}$ linked with the phase transition to a WC. These arguments suggest that measurements of the non-monotonic behavior of $I_P$ could provide a probe of the WC phase transition.
